# Supplementary material for: Learning Monocular Depth by Distilling Cross-domain Stereo Networks
Source: arXiv:1808.06586 source file (2018-08-20)
Supplement: Supplementary file 1 [file supp.pdf]

# Learning Monocular Depth by Distilling Cross-domain Stereo Networks Supplementary Material

## 1 More Visualization Results on KITTI

In Fig. 1 and 2, we demonstrate more visualization results of our models on KITTI dataset [4]. The depth ground truth is obtained by interpolating sparse LIDAR depth map.

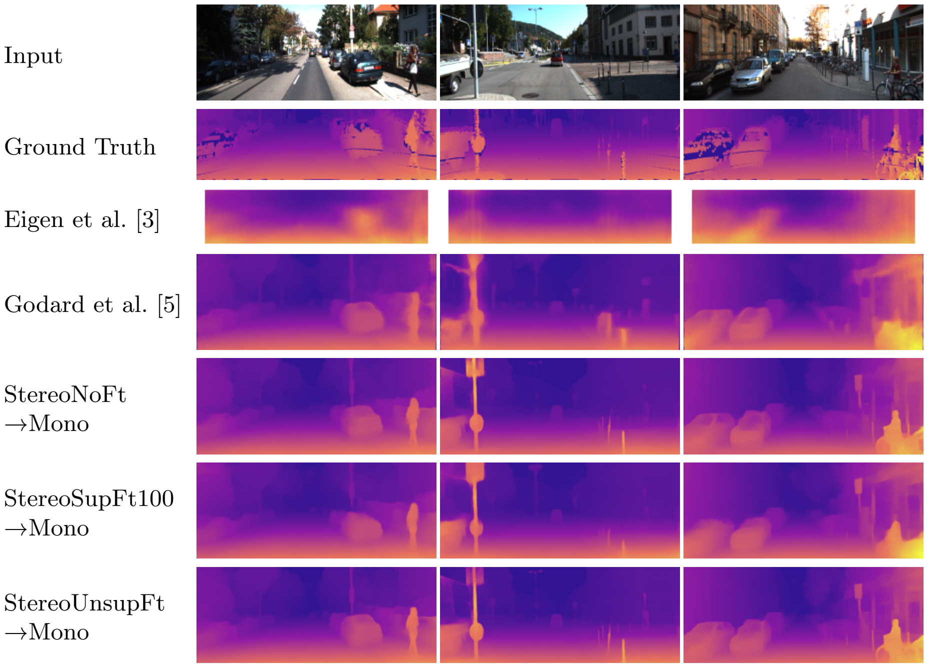


**Fig. 1.** Visualization results of our models on KITTI dataset. The ground truth is obtained from sparse LIDAR depth map by nearest neighbor interpolation.

## 2 Visualization Results on Cityscapes

In Fig. 3, we show visualization results of our monocular depth model *StereoNoFt→Mono* trained on Cityscapes dataset [2].

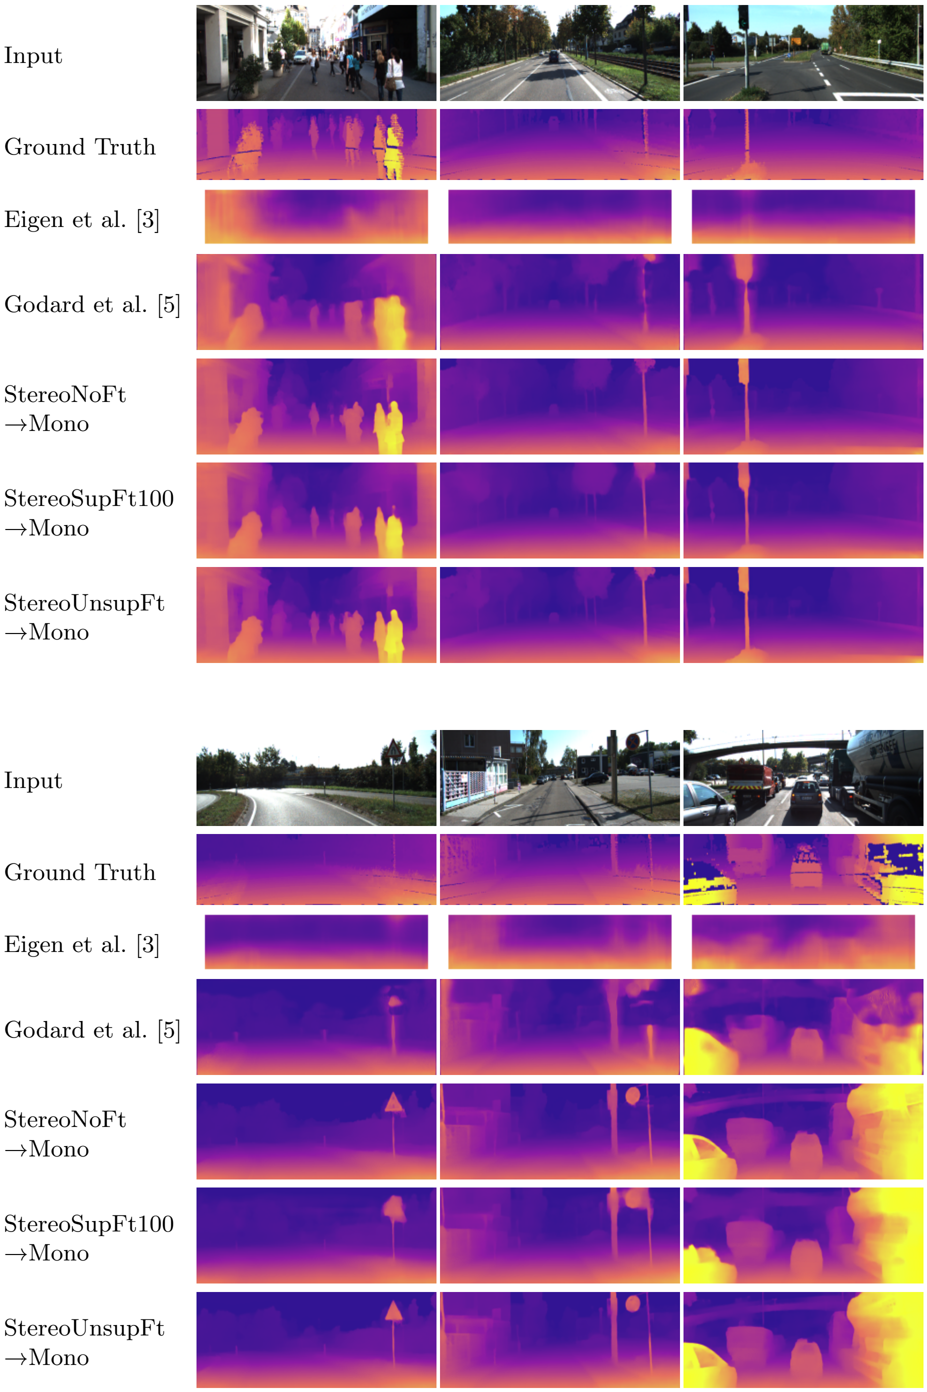


**Fig. 2.** Visualization results of our models on KITTI dataset. (Continued)

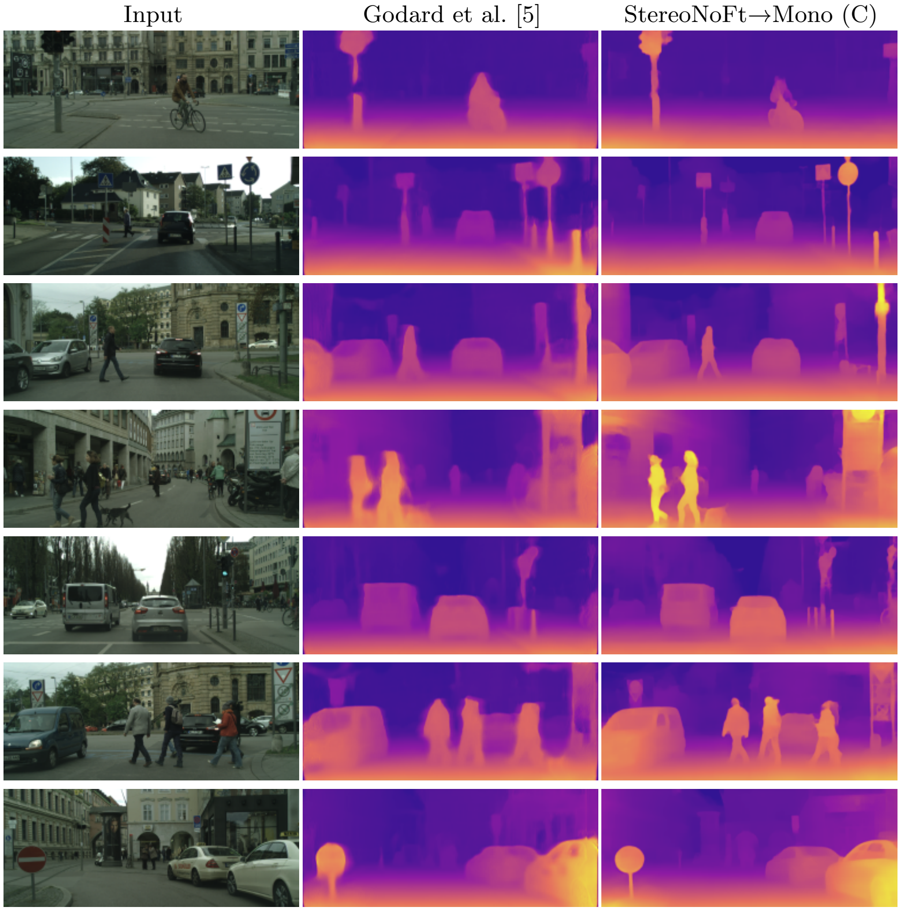


**Fig. 3.** Visualization results on Cityscapes dataset. *(C)* denotes that the monocular network is trained on Cityscapes dataset.

## 3 PSMNet as the Proxy Stereo Network

We tested our pipeline with a more advanced proxy stereo network PSMNet [1] and compared the final monocular depth results with those using DispNetC. Instead of using correlation to build up cost volume for stereo matching, PSMNet concatenates the left-right feature maps for all disparity levels to form a 4-D volume, then a stack hourglass 3D convolution network is used to aggregate the volume to predict the final disparity map.

In Table 1, we compared the performance of our method using DispnetC or PSMNet as the proxy stereo network. We can see for both supervised and unsupervised settings, using PSMNet as the proxy stereo network gives more accurate monocular depth results. As a result, the performance of our method increases with the performance of the stereo algorithm.

**Table 1.** Results on KITTI [4] with PSMNet [1] as the Proxy Stereo Network

| Method | Sup. | Dataset | lower is better | | | | higher is better | | |
|---|---|---|---|---|---|---|---|---|---|
| | | | Abs Rel | Sq Rel | RMS | Log RMS | $\delta <$ 1.25 | $\delta <$ $1.25^2$ | $\delta <$ $1.25^3$ |
| StereoUnsupFt→Mono pt | No | S,K→K | 0.099 | 0.745 | 4.424 | 0.182 | 0.884 | 0.963 | 0.983 |
| StereoUnsupFt(PSM)→Mono pt | No | S,K→K | 0.097 | 0.706 | 4.318 | 0.179 | 0.887 | 0.964 | 0.984 |
| StereoSupFt100→Mono pt | 100 | S,K→K | 0.101 | 0.690 | 4.254 | 0.173 | 0.884 | 0.966 | 0.986 |
| StereoSupFt100(PSM)→Mono pt | 100 | S,K→K | 0.092 | 0.622 | 4.249 | 0.172 | 0.885 | 0.965 | 0.986 |

## References

1. Chang, J.R., Chen, Y.S.: Pyramid stereo matching network. In: Proceedings of the IEEE Conference on Computer Vision and Pattern Recognition. pp. 5410–5418 (2018)
2. Cordts, M., Omran, M., Ramos, S., Rehfeld, T., Enzweiler, M., Benenson, R., Franke, U., Roth, S., Schiele, B.: The cityscapes dataset for semantic urban scene understanding. In: Proc. of the IEEE Conference on Computer Vision and Pattern Recognition (CVPR) (2016)
3. Eigen, D., Puhrsch, C., Fergus, R.: Depth map prediction from a single image using a multi-scale deep network. In: Advances in neural information processing systems. pp. 2366–2374 (2014)
4. Geiger, A., Lenz, P., Stiller, C., Urtasun, R.: Vision meets robotics: The kitti dataset. International Journal of Robotics Research (IJRR) (2013)
5. Godard, C., Mac Aodha, O., Brostow, G.J.: Unsupervised monocular depth estimation with left-right consistency. In: CVPR. vol. 2, p. 7 (2017)
